# Supplementary material for: Graph Enabled Cross-Domain Knowledge Transfer
Source: arXiv:2304.03452 source file (2023-07-08)
Supplement: Supplementary file 1 [file appendix.tex]

\chapter{CELL SIGNALING SITES \& PROTEIN DATABASES}
something\cite{eiglearn}
